# Supplementary material for: Turbo: Effective Caching in Differentially-Private Databases
Source: arXiv:2306.16163 source file (2023-10-23)
Supplement: Supplementary file 1 [file appendix-adhoc.tex]

\section{Ad-hoc proof}

\begin{theorem} \pmwbypass preserves $\epsilon_G$-DP, for a global privacy budget set upfront in the $\textproc{PrivacyAccountant}$.
\end{theorem}
\begin{proof}
    \pierre{This proof extends the original proof to account for concurrent composition.}

    Consider an adversary $\mathcal{A}$ that gives two neighboring datasets $x^0$ and $x^1$. Note $V^0$ the random variable representing the output of the \A\ref{alg:pmw-bypass} on $x^0$, and $V^1$ the view of the adversary on $x^1$.

    Consider $r \ge 0$ and a valid outcome $v = (v_1, \dots, v_r)$. Note $v_{<i} = (v_1, \dots, v_{i-1})$.
    The privacy loss function is defined by:

    $$Loss(v) = \ln \left(\frac{\Pr[V^0 = v]}{\Pr[V^1 = v]} \right) = \ln \left( \prod_{i=1}^r\frac{\Pr[V^0_i = v_i \vert v_{<i}] }{\Pr[V^1_i = v_i \vert v_{<i}]} \right) $$

    For all $i$ we have $v_i \in \mathbb{R} \cup \{\bot, \top\}$. We note $I_{SV} := \{ i \in [r]: v_i \in  \{\bot, \top\}\}$ and $I_{Lap} := \{ i \in [r]: v_i \in \mathbb{R} \}$.
    We further split $I_{SV}$ into a set of sparse vectors $I_{SV} = \sqcup_{k = 1}^m SV_{k}$.
    The SV are potentially interleaving, but we order them by index of the first query (\ie $\min SV_1 < \min SV_2 \dots < \min SV_m$).

    Moreover, the choice of using the Bypass branch at time $i$ only depends (deterministically) on past results $v_{<i}$, \ie if we know that $i \in I_{SV}$ then $V_i$ is the random variable corresponding to an SV output, and if $i \in I_{Lap}$ then $V_i = q_i(D) + Z_i$ for a Laplace variable $Z_i$ calibrated to have budget $\epsilon_i(v_{<i})$. We emphasize that the budget $\epsilon_i$ can depend on past results.

    Let's bound the loss by splitting it into different parts:

    \begin{align*}
        |Loss(v)| & \le \sum_{k = 1}^m |\ln(\prod_{i \in SV_k }\frac{\Pr[V^0_i = v_i \vert v_{<i}] }{\Pr[V^1_i = v_i \vert v_{<i}]} )| \\
                  & +\sum_{i \in I_{Lap}} | \ln(\frac{\Pr[ q_i(D) + Z_i = v_i \vert v_{<i}] }{\Pr[ q_i(D') + Z_i = v_i \vert v_{<i}]})
    \end{align*}

    For $i \in I_{Lap}$, we have $\ln(\frac{\Pr[ q_i(D) + Z_i = v_i \vert v_{<i}] }{\Pr[ q_i(D') + Z_i = v_i \vert v_{<i}]}) \le \epsilon_i(v_{<i})$. The previous outcomes $v_{<i}$ only affect the parameter $\epsilon_i$ of $Z_i$.

    For $k \in [m]$, we have a noisy threshold $\rho_k$. For each $i \in SV_k$, $V_i = \top$ iif $q_i(D) + \nu_i \ge T_i + \rho_k$ for the local noise $\nu_i$.
    % \pierre{I'm using the notation from \cite{lyu_sv}, will re-define if we keep this.}
    Take $i \in SV_k$. Note that under the condition that it is an SV output, $V_i$ only depends on $q_i(D), T, \nu_i$ and $\rho_k$. Moreover, $\rho_k$ only affects $v_j, j \in SV_k$.
    We note $SV_k = \{j_1, \dots, j_\ell, \dots, j_{m_k} \}$ with $j_1 < j_2 < \dots$ and $j_\ell = i$.

    Thus we can remove the conditioning on all the other outputs, apart from the fact that $V_i$ is an SV call \pierre{(we know that $V_i$ is a SV because of potentially $v_{i-1}$)}:

    $$\Pr[V^0_i = v_i \vert v_{<i}] = \Pr[V^0_i = v_i \vert v_{j_1}, v_{j_2}, \dots, v_{j_{\ell - 1}}, i \in SV_k ]$$

    \pierre{But can't we say that for any interactive mechanism, thus proving concurrent composition? That sounds too easy...?}
    \ml{is there separation examples, or at least examples of ways this cannot clearly be ruled out in the interactive DP literature? I think I'm really missing why things are (or at least could be) different under interactive mechanisms...}
    \ml{I feel like a key points might be if internal stull in the interactive mechanism can depend on the past (and hence interlieved queries). In SV, the key step seems to be upper-bouding sensitivity by a constant that doesn't depend on the past, and setting the threshold at the very beginning, which means the interlieved queries don't impact the likelyhood ratio and the can more it at the end. Another is that the interactive mechanism has budget fixed and consumed in advance. Are any of those broken in an way with other mechanisms? Could there be some early stopping stuff (like the interactive mechanism is an odometer like thing, or relies on some two steps + composition, like estimating the range and then truncating and things can amplify if you get extra information?)}
    Hence we get a simple SV transcript, where $\tilde V^0$ is the view of the adversary on a vanilla SV:
    %  (technically we can't reuse $V^0_i$ because they don't even have the same output space, when we removed the conditioning we also removed the public data that was asking us whether to use the SV or the Bypass branch):

    $$
        \prod_{i \in SV_k }\Pr[V^0_i = v_i \vert v_{<i}] = \Pr[\forall j \in [m_k], \tilde V^0_j = \tilde v_j]$$

    Thanks to \Thm 2 of \cite{lyu_sv}, $ \Pr[\forall j \in [m_k], \tilde V^0_j = \tilde v_j] \le \exp(3\epsilon_k(v_{<i_k}))  \Pr[\forall j \in [m_k], \tilde V^1_j = \tilde v_j]$.
    Where the SV parameter $\epsilon_k(v_{<i_k})$ only depends on queries answered {\em before the SV initialization}.

    Hence:

    $$|Loss(v)| \le \sum_{k = 1}^m 3\epsilon_k + \sum_{i \in I_{Lap}} \epsilon_i$$

    Finally, this view $v$ is a valid output of the algorithm, so in particular the filter allowed each mechanism to run (by paying upfront for the privacy cost). Hence $\sum_{k = 1}^m 3\epsilon_k + \sum_{i \in I_{Lap}} \epsilon_i \le \epsilon_G$ which concludes the proof.

    % Note $SV_{k,\bot} := \{i \in SV_k: v_i = \bot\}$ and $SV_{k,\top} := \{i \in SV_k: v_i = \top\}$. We have:

    % \begin{align*}
    %     \prod_{i \in SV_k }\frac{\Pr[V^0_i = v_i \vert v_{<i}] }{\Pr[V^1_i = v_i \vert v_{<i}]} & = \prod_{i \in SV_{k,\bot} } \frac{\Pr[q_i(D) + \nu_i < T_i + \rho_k | v_{<i}]}{\Pr[q_i(D') + \nu_i < T_i + \rho_k | v_{<i}]}         \\
    %                                                                                             & \cdot \prod_{i \in SV_{k,\top} } \frac{\Pr[q_i(D) + \nu_i \ge T_i + \rho_k | v_{<i}]}{\Pr[q_i(D') + \nu_i \ge T_i + \rho_k | v_{<i}]}
    % \end{align*}

    % \pierre{I can almost reuse the SV proof right away, but I want to show clearly why the $v_{<i}$ don't matter.}

    % For $i \in  SV_{k,\bot}$, we have:

    % \begin{align*}
    %     \prod_{i \in SV_{k,\bot} } \Pr[q_i(D) + \nu_i < T_i + \rho_k | v_{<i}] & = \int_{-\infty}^{\infty} \Pr[\rho_k = z]
    % \end{align*}

    % $\rho_k$ can impact older results hmm.

\end{proof}

\begin{theorem}
    Ad-hoc RDP case.
\end{theorem}

\begin{proof}

    Take an order $\alpha$.
    We have:
    $$\exp((\alpha - 1) D_\alpha(V^0 \| V^1)) = \E_{v \sim V^1} \left[\left(\frac{\Pr[V^0 = v]}{\Pr[V^1 = v]} \right)^\alpha \right]$$

    Like above, we can rewrite:
    $$\Pr[V^0 = v] = \prod_{k = 1}^m \Pr[\forall i \in [|SV_k|], \tilde V^0_i = \tilde v_i] \cdot \prod_{i \in I_{Lap}} \Pr[ q_i(D) + Z_i = v_i]$$

    \pierre{Redo the RDP filter proof? Swap the integrals, etc.}

\end{proof}
