# Supplementary material for: Turbo: Effective Caching in Differentially-Private Databases
Source: arXiv:2306.16163 source file (2023-10-23)
Supplement: Supplementary file 2 [file appendix-general-concurrent-related.tex]

We first re-state existing definitions.
\subsection{Concurrent composition of interactive mechanisms (copied from \cite{vadhan_interactive}).}

\newcommand{\View}{\mathrm{View}}
\newcommand{\concomp}{{\text{ConComp}}}
\begin{definition}[Concurrent composition of interactive mechanisms]
    \label{def:concomp}
    Let $\mathcal{M}_1,\ldots, \mathcal{M}_{k}$ be interactive mechanisms. $\mathcal{M}=ConComp(\mathcal{M}_1,\ldots, \mathcal{M}_{k})$ is the concurrent composition of mechanisms $\mathcal{M}_1,\ldots, \mathcal{M}_{k}$ defined as follows:
    \begin{enumerate}
        \item Random sample $r=(r_1,\ldots,r_{k})$ where $r_j$ are random coin tosses for $\mathcal{M}_j$.
        \item Inputs for $\mathcal{M}$ consists of $x=(x_1,\ldots,x_{k})$ where $x_j$ is a private dataset for $\mathcal{M}_j$.
        \item $\mathcal{M}(x,m_0,\ldots,m_{i-1};r)$ is defined as follows:
              \begin{enumerate}
                  \item Parse $m_{i-1}$ as $(j,q)$ where $j=1, \ldots, k$ and $q$ is a query to $\mathcal{M}_j$. If $m_{i-1}$ cannot be parsed correctly, output $\texttt{halt}$.
                  \item Extract history $(m_0^j,\ldots,m_{t-1}^j)$ from $(m_0,\ldots,m_{i-1})$ where $m_i^j$ are all of the queries to mechanism $\mathcal{M}_j$.
                  \item Output $\mathcal{M}_j(x_j, m_0^j,\ldots,m_{t-1}^j; r_j)$.
              \end{enumerate}
    \end{enumerate}
    For an adversary $A$, we will use the notation $\View(A\leftrightarrow (\mathcal{M}_1,\ldots, \mathcal{M}_{k}))$ as shorthand for $\View(A\leftrightarrow \concomp(\mathcal{M}_1,\ldots, \mathcal{M}_{k}))$
\end{definition}

\subsection{Composition of non-interactive mechanisms with adaptively chosen parameters (copied from \cite{rogers2016privacy}).}

\pierre{TODO: harmonize notation a bit.}

\newcommand{\cA}{\mathcal{A}}

\newcommand{\game}{\ensuremath{\mathtt{AdaptParamComp}}}
\newcommand{\filtgame}{\ensuremath{\mathtt{PrivacyFilterComp}}}

\newcommand{\filt}{\ensuremath{\mathtt{F}}}

\newcommand{\bbx}{\mathbf{x}}
\newcommand{\cM}{\mathcal{M}}
\newcommand{\compfilt}{\ensuremath{\mathtt{COMP}}}
\newcommand{\halt}{\ensuremath{\mathtt{HALT}}}

% The view of the interaction is the tuple that includes $\cA$'s random coin tosses $R_\cA$ and the outcomes $A = (A_1, \cdots, A_k)$ of the algorithms she chose. Formally, we define an \emph{adaptively chosen privacy parameter composition game} in \ref{alg:game} which takes as input an adversary $\cA$, a number of rounds of interaction $k$, and an experiment parameter $b \in \{0,1\}$.
\begin{algorithm}[h!]
    \caption{$\game(\cA,k,b)$}
    \label{alg:game}
    \begin{algorithmic}
        \State Select coin tosses $R_\cA$ for $\cA$ uniformly at random.
        \For{$i = 1,\cdots, k$}
        \State $\cA = \cA(R_\cA,A_1^b,\cdots, A_{i-1}^b)$ gives neighboring $\bbx^{i,0}, \bbx^{i,1}$, parameters $(\epsilon_i, \delta_i)$,  $\cM_i$ that is $(\epsilon_i,\delta_i)$-DP
        \State$\cA$ receives $A^b_i = \cM_i(\bbx^{i,b})$
        \EndFor
        \Return view $V^b = (R_\cA, A_1^b, \cdots, A_k^b)$
    \end{algorithmic}
\end{algorithm}

\begin{algorithm}
    \caption{$\filtgame(\cA,k,b; \compfilt_{\epsilon_g,\delta_g})$}
    \label{alg:filter_game}
    \begin{algorithmic}
        \State Select coin tosses $R_\cA^b$ for $\cA$ uniformly at random.
        \For{$i = 1,\cdots, k$}
        \State {$\cA = \cA(R^b_\cA,A_1^b,\cdots, A_{i-1}^b)$ gives neighboring $\bbx^{i,0}, \bbx^{i,1}$,  $(\epsilon_i, \delta_i)$, and $\cM_i$ that is $(\epsilon_i,\delta_i)$-DP}
        \If{$\compfilt_{\epsilon_g,\delta_g}\left( \epsilon_1,\delta_1,\cdots, \epsilon_i,\delta_i, 0,0,\cdots, 0,0\right) = \halt$}
        \State $A_i, \cdots, A_k = \bot$
        \State BREAK
        \Else{}
        \State{$\cA$ receives $A^b_i = \cM_i(\bbx^{i,b})$ }
        \EndIf
        \EndFor
        \Return view $V_\filt^b = (R^b_\cA, A_1^b, \cdots, A_k^b)$
    \end{algorithmic}
\end{algorithm}

The problem with this algorithm is that it only works for non-interactive mechanisms, \ie the adversary receives the full output of mechanism $i$ at round $i$, and then sequentially calls the next mechanisms without ever communicating with $cM_i$ again.
